# Supplementary material for: Measurement of $C\!P$-averaged observables in the $B^{0}\rightarrow K^{*0}\mu^{+}\mu^{-}$ decay
Source: arXiv:2003.04831 source file (2020-07-14)
Supplement: Supplementary file 1 [file appendix.tex]

{\noindent\bf\Large Supplemental Material} \\
%%% This is for arxiv - will be the appendix - rest of the projections will go in the auxiliary file
